# Supplementary material for: Realisation of Symmetry Enforced Two-Dimensional Dirac Fermions in Nonsymmorphic $\alpha$-Bismuthene
Source: arXiv:1906.08456 source file (2019-06-20)
Supplement: Supplementary file 1 [file SI_Bismuthene_v9.pdf]

# Supplementary Information: Realisation of Symmetry Enforced Two-Dimensional Dirac Fermions in Nonsymmorphic $\alpha$-Bismuthene

Pawel J. Kowalczyk, Simon A. Brown, Tobias Maerkl, Qiangsheng Lu, Ching-Kai Chiu, Ying Liu, Shengyuan A. Yang, Xiaoxiong Wang, Ilona Zasada, Francesca Genuzio, T. Onur Menteş, Andrea Locatelli, Tai-Chang Chiang, Guang Bian

## I. EXPERIMENTAL AND COMPUTATIONAL METHODS

Commercially available HOPG (SPI-1) was used as a substrate in all experiments. It was cleaved in air, then loaded into the UHV system and annealed at 700 − 900 K for several hours to remove contaminants. After the substrate cooled down to room temperature, high purity bismuth (99.999%) was evaporated from a ceramic crucible and deposited onto the substrate at rates ∼0.01 Å/s.

LEEM, $\mu$-LEED and $\mu$-ARPES measurements were performed at room temperature and base pressure of $10^{-9}$ Pa with the spectroscopic photoemission and low-energy electron microscope (SPELEEM) installed at the Nanospectroscopy beamline of the Elettra synchrotron laboratory (Italy)[1]. Soft X-rays at energy 27.9 eV were used for $\mu$-ARPES measurements. Kinetic electron energies were analyzed using hemispherical bandpass energy filter (operating with pass energy of 908 eV). 500 and 2000 nm wide apertures were used for $\mu$-LEED and $\mu$-ARPES measurements respectively.

First-principles calculations of the electronic structure of the films were performed using Hartwigsen-Goedecker-Hutter-type pseudopotentials[2] and a plane-wave basis set. The main program employed was developed by the ABINIT group[3]. Spin-orbit coupling was included using the relativistic LDA approximation.

LEED intensity calculations were performed with TensErLEED package[4]. The electron scattering was determined from the scattering phase shifts. Ten ($l_{max}$=9) phase shifts for Bi were calculated with the Barbieri/Van Hove phase shift package[5]. The number of phase shifts which have to be used in LEED calculations depends on the upper limit of the energy used in the experiment and on the atoms radiuses which form the sample[6]. The use of $l_{max} = 9$ is formally justified by the upper energy limit for which the terms in summation over $l$ give a non-zero contribution. An energy-dependent inner potential was employed in the simulation. The free standing layer of $\alpha$-Bi was simulated using the average T-matrix approximation.

## II. LEED ANALYSIS

We begin by listing the main observations from our $\mu$-LEED measurements (see Fig. 1**a** in main text):

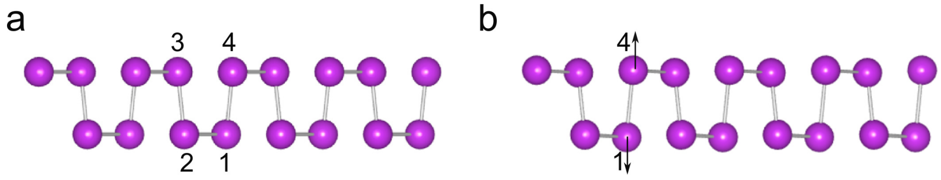


**Figure S1** **$\alpha$-Bi surface buckling. a,** The ball models of bismuthene without deformation and **b,** with atoms 1, 4 displaced. All four atoms in the unit cell are enumerated, arrows indicate atoms which were vertically displaced of their DFT calculated position.

A. the intensity of the (10) and ($\bar{1}$0) spots is small - ~10% of the intensity of the (11) spots

B. the intensity of (01) and (0$\bar{1}$) are ~42% and ~49% of the (11) spot intensity

C. the ratio of (0$\bar{1}$) and (01) intensities is 1.2

D. the uncertainty in these ratios is at the level of 25%

In order to estimate the influence of the deformation of the crystallographic structure on the LEED spot intensities we performed dynamic LEED simulations for a variety of deformed $\alpha$-Bi structures. Starting with the nonsymmorphic structure depicted in Fig. **S1a**, we displaced selected atoms and then calculated the intensity of each of the main LEED spots. The electron energy was 40 eV as in the experiments. An example of one such deformation is shown in Fig. **S1b** in which atoms 1 and 4 (see Fig. **S1a**) were displaced downward (↓) and upward (↑) respectively (i.e. 1↓4↑). We modeled all the deformations

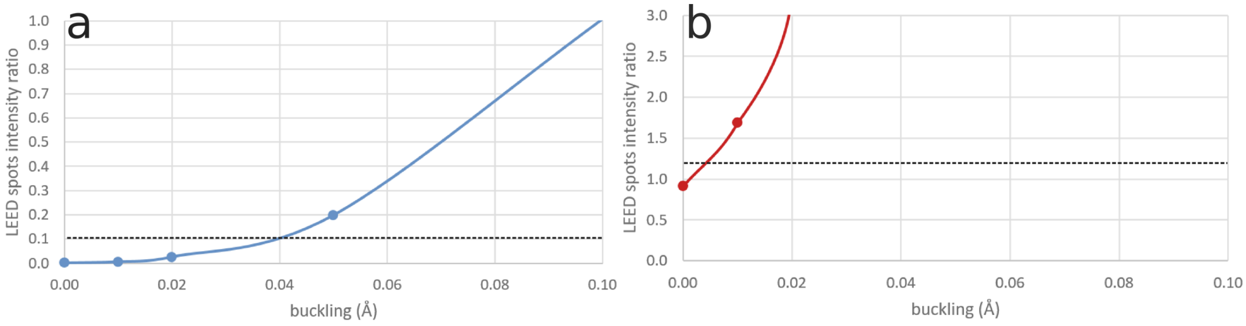


**Figure S2** **Ratio of calculated LEED spot intensity as a function of $\alpha$-Bi surface buckling. a,** (10)/(11) ratio. **b,** (0$\bar{1}$)/(01) ratio. The upper range of the experimentally measured ratios are shown using horizontal dashed lines.

1↑4↑, 1↓4↓, 2↑3↑, 2↓3↓, 1↓4↑, 2↓3↑ and obtained similar results in qualitative agreement to experimental findings for 1↓4↓, 2↑3↑, 1↓4↑.

The comparison of our LEED measurements with the theoretical calculations suggest that the buckling is small, with an upper limiton the deformation Δz around 0.04 Å. The apparent distortion in LEED might be attributed to a weak interaction with the substrate and the thermal effects. These extrinsic factors may be suppressed by optimizing the substrate condition and reducing the temperature. We simulated the band structure with a surface buckling of 0.04 Å, and the result is shown in Figure S3. The energy gap is 25 meV at $\bar{\mathrm{X}}_1$ and 29 meV at $\bar{\mathrm{X}}_2$. Let us take a closer look at the band structure. With the inclusion of distortion-induced gaps, the band dispersion is still linear along $\bar{\mathrm{X}}_1$-$\bar{\Gamma}$ and $\bar{\mathrm{X}}_2$-$\bar{\Gamma}$ in an energy window of 200 meV. Along $\bar{\mathrm{X}}_2$-$\bar{\mathrm{M}}$, the band is so anisotropic that the cone feature is overwhelmed by the gap. By contrast, the bands along $\bar{\mathrm{X}}_1$-$\bar{\mathrm{M}}$ still resemble a "gapped" cone in an energy window of 100 meV.

## III. NODAL-LINE BAND STRUCTURE OF $\alpha$-BI IN THE ABSENCE OF SPIN-ORBIT COUPLING

According to the DFT band calculation without the inclusion of SOC, there exist nodal lines along $\bar{\mathrm{X}}_1$-$\bar{\mathrm{M}}$-$\bar{\mathrm{X}}_2$. Here we show this band denegeracy is due to the nonsymmorphic symmetry of the lattice. The three generators of the space group are listed as follows:

$$\widetilde{M_z} :(x+1/2, y+1/2, -z); \tag{1}$$

$$P :(-x, -y, -z); \tag{2}$$

$$M_x :(-x, y, z). \tag{3}$$

Let $\widetilde{M_z}$ and $M_x$ act on $(x, y, z)$ in the different orders and we have:

$$(x, y, z) \xrightarrow{M_x} (-x, y, z) \xrightarrow{\widetilde{M_z}} (-x+1/2, y+1/2, -z), \tag{4}$$

$$(x, y, z) \xrightarrow{\widetilde{M_z}} (x+1/2, y+1/2, -z) \xrightarrow{M_x} (-x-1/2, y+1/2, -z). \tag{5}$$

Hence, these two combinations are connected by the momentum-dependent phase,

$$\widetilde{M_z} M_x = T_{100} M_x \widetilde{M_z}, \tag{6}$$

where $T_{100} = e^{ik_x}$ denotes the translation by one unit cell along $x$ direction. Consider a generic momentum point $\boldsymbol{k}_1 = (\pi, k)$ between $\bar{\mathrm{X}}_1$ and $\bar{\mathrm{M}}$. $T_{100} = -1$ at $\boldsymbol{k}_1$, so we have

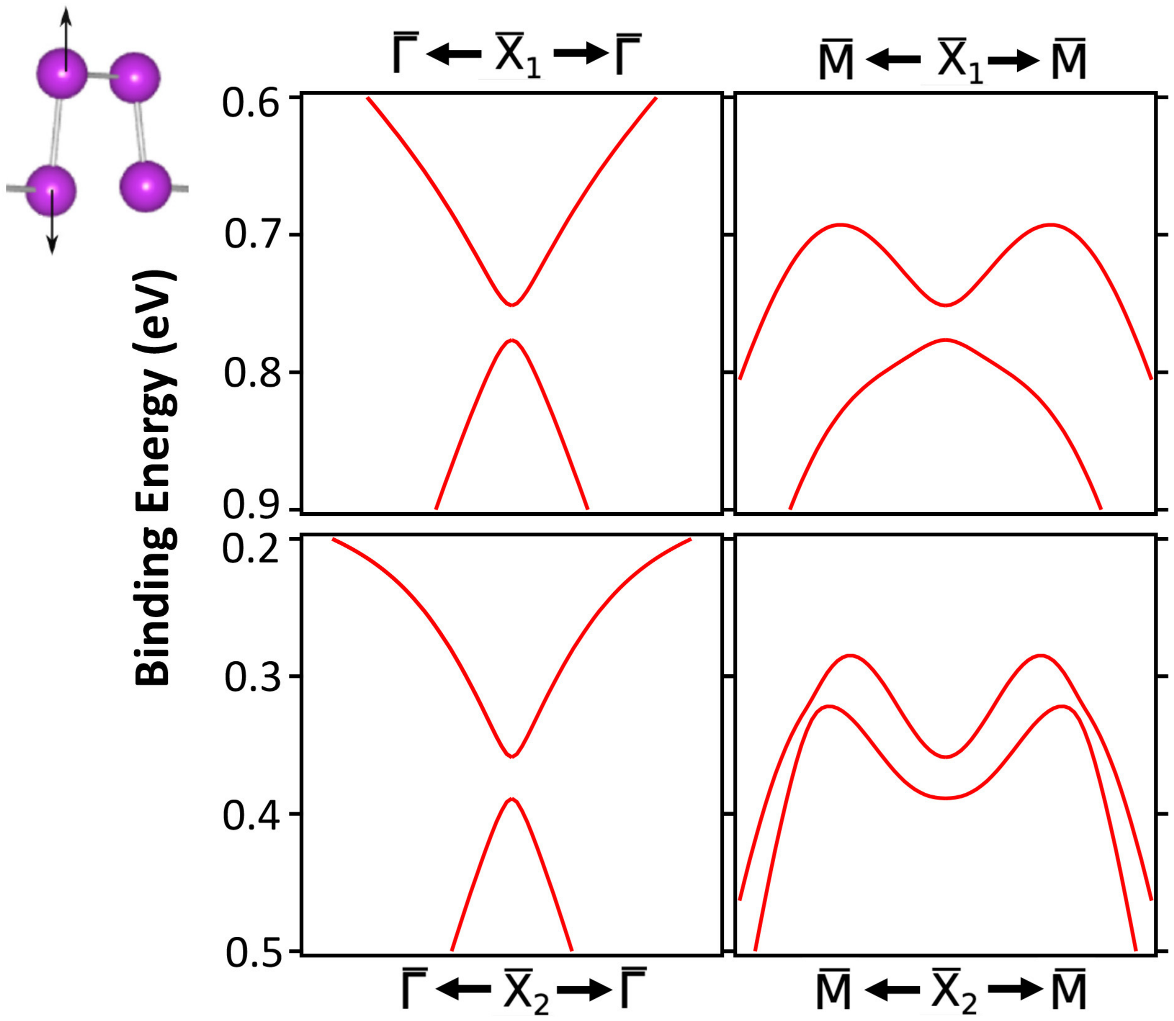


**Figure S3  Band structure of distorted $\alpha$-bismuthene.** The zoom-in band structure around $\bar{\mathrm{X}}_1$ and $\bar{\mathrm{X}}_2$ of $\alpha$-bismuthene with a surface distortion of 0.04 Å. The distortion is schematically shown at the top-left corner.

$\{\widetilde{M}_z, M_x\} = 0$. Meanwhile, $\boldsymbol{k}_1$ is invariant under the operations of $\widetilde{M}_z$ and $M_x$. We can choose an energy eigenstate $|\Phi(\boldsymbol{k}_1)\rangle$ at $\boldsymbol{k}_1$, which is also an eigenstate of $M_x$ with eigenvalue $g_x$ ($g_x$=+1 or $-1$, since we consider the mirror-reflection eigenvalue in a spinless case). From $\{\widetilde{M}_z, M_x\} = 0$, we know that $\widetilde{M}_z|\Phi(\boldsymbol{k}_1)\rangle$ must be another degenerate partner of $|\Phi(\boldsymbol{k}_1)\rangle$ with an *opposite* $M_x$ eigenvalue ($-g_x$). Therefore, the band degeneracy is 2 at every momentum between $\bar{\mathrm{X}}_1$ and $\bar{\mathrm{M}}$.

Similar proof for band degeneracy works for a generic momentum point $\boldsymbol{k}_2 = (k, \pi)$ between $\bar{\mathrm{X}}_2$ and $\bar{\mathrm{M}}$. The two symmetry operators which are responsible for the band degeneracy

are $\widetilde{M}_z$ and $\widetilde{M}_y$, where

$$\widetilde{M}_y \equiv \widetilde{M}_z P M_x : (x, y, z) \to (x + 1/2, -y + 1/2, z). \tag{7}$$

It is easy to see that

$$\widetilde{M}_z \widetilde{M}_y = T_{010} \widetilde{M}_y \widetilde{M}_z, \tag{8}$$

where $T_{010} = e^{ik_y}$ denotes the translation by one unit cell along $y$ direction. $\boldsymbol{k}_2$ is invariant under $\widetilde{M}_z$ and $\widetilde{M}_y$. The anti-commutation relation $\{\widetilde{M}_z, \widetilde{M}_y\} = 0$ at $\boldsymbol{k}_2$ leads to the two-fold band degeneracy at this momentum point.

## IV. 2D DIRAC FERMIONS IN A BISMUTH MONOLAYER STRUCTURE

To illustrate the application of the principle to other cases, we now consider a different nonsymmorphic layer group. The lattice structure of a bismuth monolayer after DFT optimization is shown in Fig. **S4a**, and it belongs to the #15 layer group ($p2_1/m11$). Note the buckling in this structure i.e. the two atoms in the unit cell are not exactly in plane, as shown in Fig. **S4a**. The layer group has two generators (with spin matrices) as follows:

$$P : (-x, -y, -z) s_0 \tag{9}$$

$$\widetilde{C}_{2x} : (x - 1/2, -y, -z) i s_x \tag{10}$$

where $\widetilde{C}_{2x}$ is a nonsymmorphic 2-fold screw axis operation. The combinations of these two operators in two different orders are given by

$$(x, y, z) \xrightarrow{P} (-x, -y, -z) \xrightarrow{\widetilde{C}_{2x}} (-x - 1/2, y, z) \tag{11}$$

$$(x, y, z) \xrightarrow{\widetilde{C}_{2x}} (x - 1/2, -y, -z) \xrightarrow{P} (-x + 1/2, y, z) \tag{12}$$

Hence, the two combinations are connected by the momentum-dependent phase,

$$P \widetilde{C}_{2x} = T_{100} \widetilde{C}_{2x} P, \tag{13}$$

where $T_{100} = e^{ik_x}$. In this case, at $\bar{\mathrm{M}} = (\pi, \pi)$ and $\bar{\mathrm{X}}_1 = (\pi, 0)$, we have $\{P, \widetilde{C}_{2x}\} = 0$. Meanwhile, the nonsymmorphic character also makes the eigenvalues of $\widetilde{C}_{2x}$ momentum-dependent. Since $(\widetilde{C}_{2x})^2 = -T_{100}$ (the minus sign is due to a $2\pi$ rotation on spin), we have the $\widetilde{C}_{2x}$ eigenvalues $c_x = \pm i e^{ik_x/2}$. Importantly, at both $\bar{\mathrm{X}}_1$ and $\bar{\mathrm{M}}$, $c_x = \pm 1$, which are

purely real. Suppose $|\Phi\rangle$ is an eigenstate of $\widetilde{C}_{2x}$ at $\bar{\mathrm{X}}_1$ (or $\bar{\mathrm{M}}$). Following a similar derivation as in the case of $\alpha$-Bi, $|\Phi\rangle$, $T|\Phi\rangle$, $P|\Phi\rangle$, and $TP|\Phi\rangle$ must be degenerate at $\bar{\mathrm{X}}_1$ (or $\bar{\mathrm{M}}$). This is indeed the case we find in the calculated band structure of the bismuth monolayer shown in Fig. S4**b**.

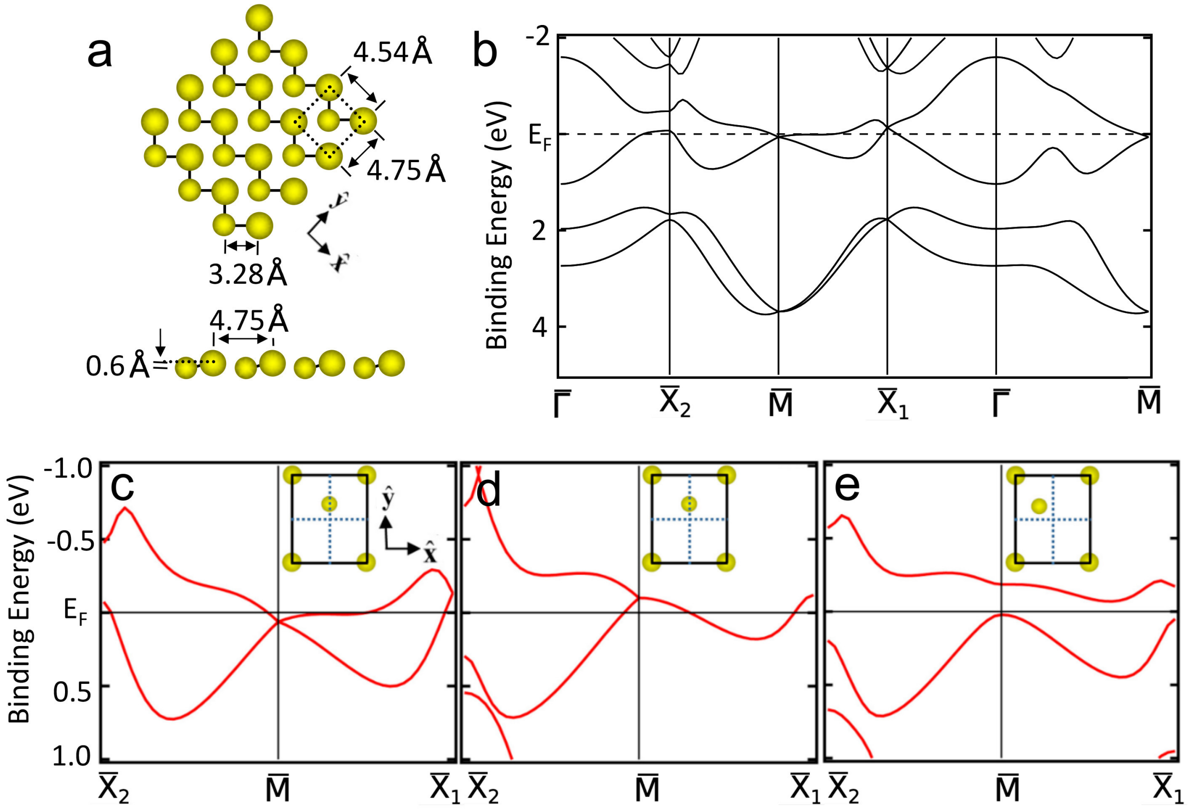


**Figure S4 Lattice and band structure of bismuth monolayer. a,** The top and side views of Bi monolayer lattice structure. **b,** DFT band structure of Bi monolayer. **c,** Zoom-in band structure along $\bar{\mathrm{X}}_2$-M-$\bar{\mathrm{X}}_1$. The lattice is shown in the inset. **d,** Band structure same as in **c** but calculated in the absence of spin-orbit coupling. **e,** Bands calculated with a distorted lattice. The distortion is schematically shown in the inset.

In the absence of spin-orbit coupling, the bands are degenerate and become line nodes along $\bar{X}_1 - \bar{\mathrm{M}}$, see Fig. **S4d**. To see this, let us consider two operators $M_x$ and $C_t$, where

$$M_x \equiv \widetilde{C}_{2x}P : (x, y, z) \rightarrow (-x - 1/2, y, z) \tag{14}$$

$$C_t \equiv \widetilde{C}_{2x}T : (x, y, z) \rightarrow (x - 1/2, -y, -z) \tag{15}$$

Following a similar derivation as in Equations. (11) and (12), we have $M_x C_t = T_{100} C_t M_x$, where $T_{100} = e^{ik_x}$. A generic momentum point $\boldsymbol{k} = (\pi, k_y)$ between $\bar{\mathrm{X}}_1$ and $\bar{\mathrm{M}}$ is invariant under $M_x$ and $C_t$, since $k_y$ changes its sign under $\widetilde{C}_{2x}$, $P$, and $T$. Meanwhile, $\{M_x, C_t\} = 0$ at $\boldsymbol{k}$. This anti-commutation relation guarantees the 2-fold band degeneracy at $\boldsymbol{k}$, which leads to a nodal line along $\bar{\mathrm{X}}_1$-$\bar{\mathrm{M}}$ in the absence of SOC. Therefore, SOC is crucial for the formation of the Dirac cone. The Dirac bands found in this Bismuth structure are intrinsically of spin-orbit origin, in contrast to the spinless Dirac states in graphene. Just like the case of $\alpha$-Bi, the band crossing point is protected by the nonsymmorphic lattice symmetry which eliminates the gap-opening effect of spin-orbit coupling in this 2D material. Consequently, breaking lattice symmetry will naturally introduce an energy gap at the Dirac point, as illustrated in Fig. **S4e**, which provides a tunability of the electronic property of this family of 2D Dirac materials. We note that the Dirac states are very close the Fermi level, so this Bi monolayer is a 2D Dirac semimetal. This structure is not energetically favored in its free-standing form, but it can be stabilized with the aid of substrate interactions[7].

## V. COMPARISON OF $\mu$-ARPES SPECTRA TAKEN FROM HOPG AND FROM $\alpha$-BI GROWN ON HOPG

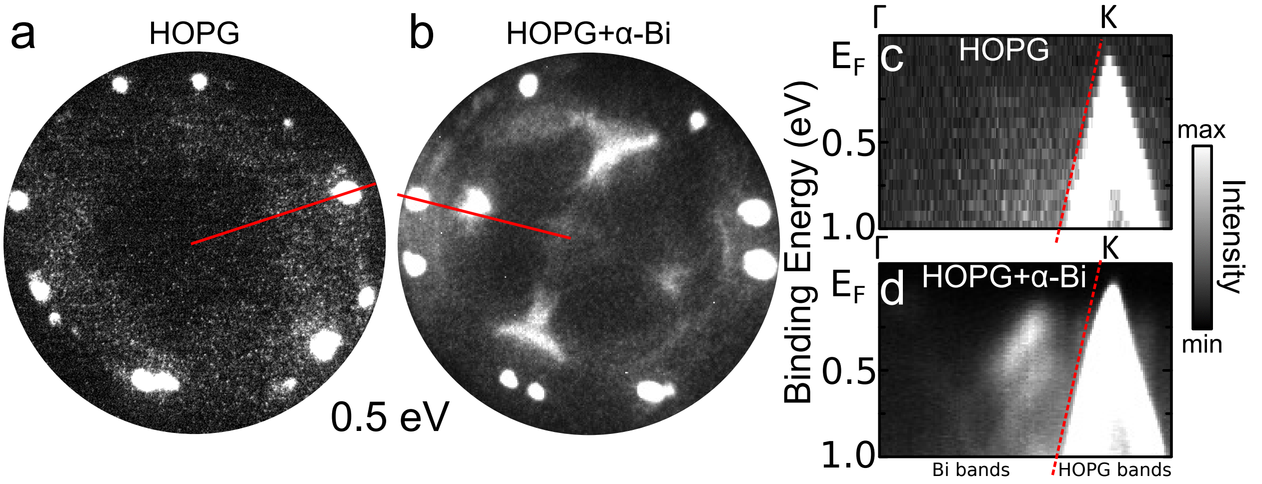


**Figure S5** **$\mu$-ARPES spectra of HOPG and $\alpha$-Bi. a-b,** $\mu$-ARPES iso-energy contours taken at photon energy 28.0 eV and binding energy 0.5 eV on the domains of HOPG and $\alpha$-Bi (grown on HOPG). **c-d,** The band mapping along red lines shown in **a** and **b**.

It is well known that HOPG band structure in vicinity to the Fermi level is characterized by the presence of bands only around K point[12]. There are no valence bands with binding energy less than 4 eV near the center of the Brillouin zone[12]. Moreover, small interatomic distances between carbon atoms result in a relatively large 1$^{st}$ BZ for HOPG. By contrast, interatomic distances of $\alpha$-Bi are much larger, which results in a smaller 1$^{st}$ BZ. Therefore, HOPG is an ideal candidate as a substrate for ARPES measurements on Bi because there are no HOPG bands interfering with Bi ones. This is illustrated in Fig. **S5** in which we show the $\mu$-ARPES spectra taken from HOPG and $\alpha$-Bi grown on HOPG (note, both measurements were conducted on the same sample). It is clear that there is no bands around $\Gamma$ point in the HOPG data (see Fig. **S5a** and Fig. **S5c**). By contrast, in the $\alpha$-Bi data (see Fig. **S5b** and Fig. **S5d**), one observes rich electronic structure at the center of the 1$^{st}$ BZ. All bands showing up between $\Gamma$ point and red dashed lines indicated in Fig. **S5c** and Fig. **S5d** are intrinsic to $\alpha$-Bi. Therefore, there is little overlap in the valence bands near the Fermi level between $\alpha$-Bi and HOPG. Previously, we have shown that there is no chemical bond forming between Bi and HOPG[13]. Furthermore, the lattices of $\alpha$-Bi and HOPG are incommensurate in both lattice constants and lattice symmetry. Therefore, the Bi film can be treated as a nearly free standing layer with only van der Waals-type substrate interactions[14].

## VI. SYMMETRY ARGUMENT FOR NONSYMMORPHIC STRUCTURE

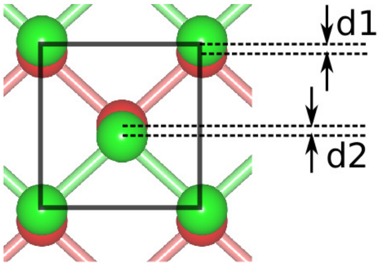


**Figure S6 Definition of in-plane separation between atoms in Bi(110).**

The nonsymmorphic $\alpha$-Bi structure can be regarded as a variation of atomic layers truncated along (110) direction from Bi bulk lattice. In the Bi bulk structure, the atoms form a rhombohedral lattice. Therefore, if we look at (110) surface unit cell, d1 is generally not equal to d2 (see Fig. **S6** for d1 and d2 definition) and the structure violates the nonsymmorphic symmetry. In 2D there is no constraint from the bulk lattice, so the atoms arrange

their positions to saturate the dangling orbital of both atoms in the unit cell in the same way. Therefore, the pair of Bi atoms at the corner of the unit cell should be equivalent to the pair at the center. In other words, d1= d2. This naturally leads to a nonsymmorphic structure in $\alpha$-Bi and other group-V element monolayers (such P[8,9] and Sb[10,11]).

## VII. GLIDED MIRROR SYMMETRY IN $\alpha$-BI AND SCREW AXIS IN MONOLAYER BI

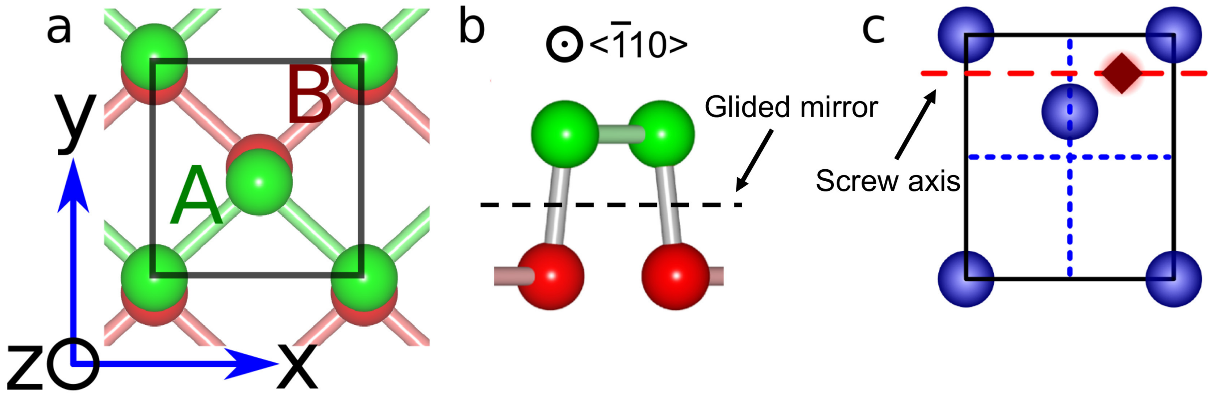


**Figure S7 Lattices for $\alpha$-Bi and monolayer Bi. a,** Top view of $\alpha$-Bi. The two sublayers (red and green) sit at different $z$ planes. **b,** Side view of $\alpha$-Bi. The glided mirror plane is parallel to the $x-y$ plane, as marked by the black dashed line. **c,** Lattice of monolayer Bi with the inversion center indicated by the red diamond. The screw axis passes the inversion center as marked by the red dashed line.

### A. Glided mirror symmetry in $\alpha$-Bi

There are two flat atomic layers (green and red in Fig. **S7a**) sitting at different $z$ planes. The mirror is parallel to the $x$-$y$ plane and in between the two atomic layers, see the side view in Fig. **S7b**. If we do the mirror reflection and then shift the lattice by $(a_x/2, a_y/2)$, the lattice stays same. Note that the horizontal separation between green ball A and red ball B in Fig. **S7a** is $(a_x/2, a_y/2)$.

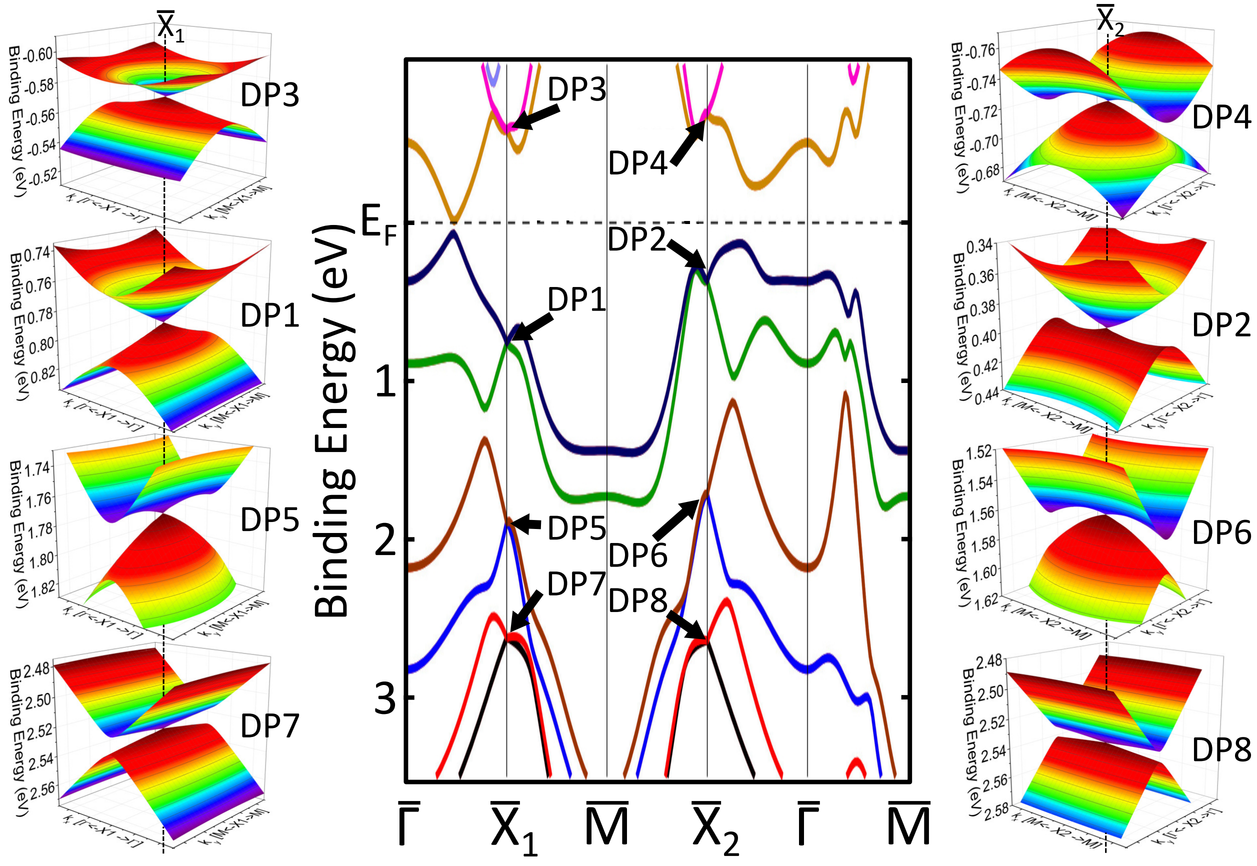


**Figure S8 Band diagram for $\alpha$-Bi.**

### B. Screw axis in monolayer Bi

There are two atomic sublayers sitting at different $z$ planes (see Fig. **S7c** and Fig. **S4a**). The inversion center sits in middle of the two Bi atoms, marked by the red diamond. The screw axis passes this inversion center and is along the x direction, shown by the red dashed line. If we rotate the lattice with respect to this axis by 180° and then shift the lattice by $(a_x/2, 0)$, the lattice stays same. So the red line is a screw axis.

## VIII. DIRAC POINTS AT $\bar{X}_1$ AND $\bar{X}_2$

In Fig. **S8** we show that multiple Dirac Points are observed at the $\bar{X}_1$ and $\bar{X}_2$ high symmetry points (see DFT band surfaces calculated in vicinity of $\bar{X}_1$ and $\bar{X}_2$ labeled DP1 -

DP8 in Fig. **S8**).


[1] Menteş, T. O., Zamborlini, G., Sala, A. & Locatelli, A. Cathode lens spectromicroscopy: methodology and applications. *Beilstein J. Nanotechnol.* **5**, 1873–1886 (2014).

[2] Hartwigsen, C., Goedecker, S. & Hutter, J. Relativistic separable dual-space gaussian pseudopotentials from H to Rn. *Phys. Rev. B* **58**, 3641–3662 (1998).

[3] Gonze, X. *et al.* First-principles computation of material properties: the ABINIT software project. *Comput. Mater. Sci.* **25**, 478–492 (2002).

[4] Blum, V. & Heinz, K. Fast LEED intensity calculations for surface crystallography using tensor LEED. *Comput. Phys. Commun.* **134**, 392–425 (2001).

[5] Barbieri, A. & Hove, M. A. V. Private communication.

[6] Van Hove, M. A., Weinberg, W. H. & Chan, C.-M. *Low-Energy Electron Diffraction* (Springer-Verlag, 1986).

[7] Kowalczyk, P. J. *et al.* Single atomic layer allotrope of bismuth with rectangular symmetry. *Phys. Rev. B* **96**, 205434 (2017).

[8] Li, P. & Appelbaum, I. Electrons and holes in phosphorene. *Phys. Rev. B* **90**, 115439 (2014).

[9] Wu, Q. *et al.* Electronic and transport properties of phosphorene nanoribbons. *Phys. Rev. B* **92**, 035436 (2015).

[10] Shi, Z.-Q. *et al.* Van der Waals heteroepitaxial growth of monolayer Sb in a puckered honeycomb structure. *Adv. Mater.* **31**, 1806130 (2018).

[11] Maerkl, T. *et al.* Engineering multiple topological phases in nanoscale Van der Waals heterostructures: realisation of $\alpha$-antimonene. *2D Mater.* **5**, 011002 (2017).

[12] Zhou, S. Y. *et al.* Coexistence of sharp quasiparticle dispersions and disorder features in graphite. *Phys. Rev. B* **71**, 161403 (2005).

[13] Kowalczyk, P. J. *et al.* STM and XPS investigations of bismuth islands on HOPG. *Surf. Sci.* **605**, 659 – 667 (2011).

[14] Kowalczyk, P. J. *et al.* Electronic size effects in three-dimensional nanostructures. *Nano Lett.* **13**, 43–47 (2013).
